# Supplementary material for: Novel-view Synthesis and Pose Estimation for Hand-Object Interaction from Sparse Views
Source: arXiv:2308.11198 source file (2023-08-22)
Supplement: Supplementary file 1 [file sup_joint.tex]

\begin{figure}[h]
\centering%
\includegraphics[width=0.8\linewidth]{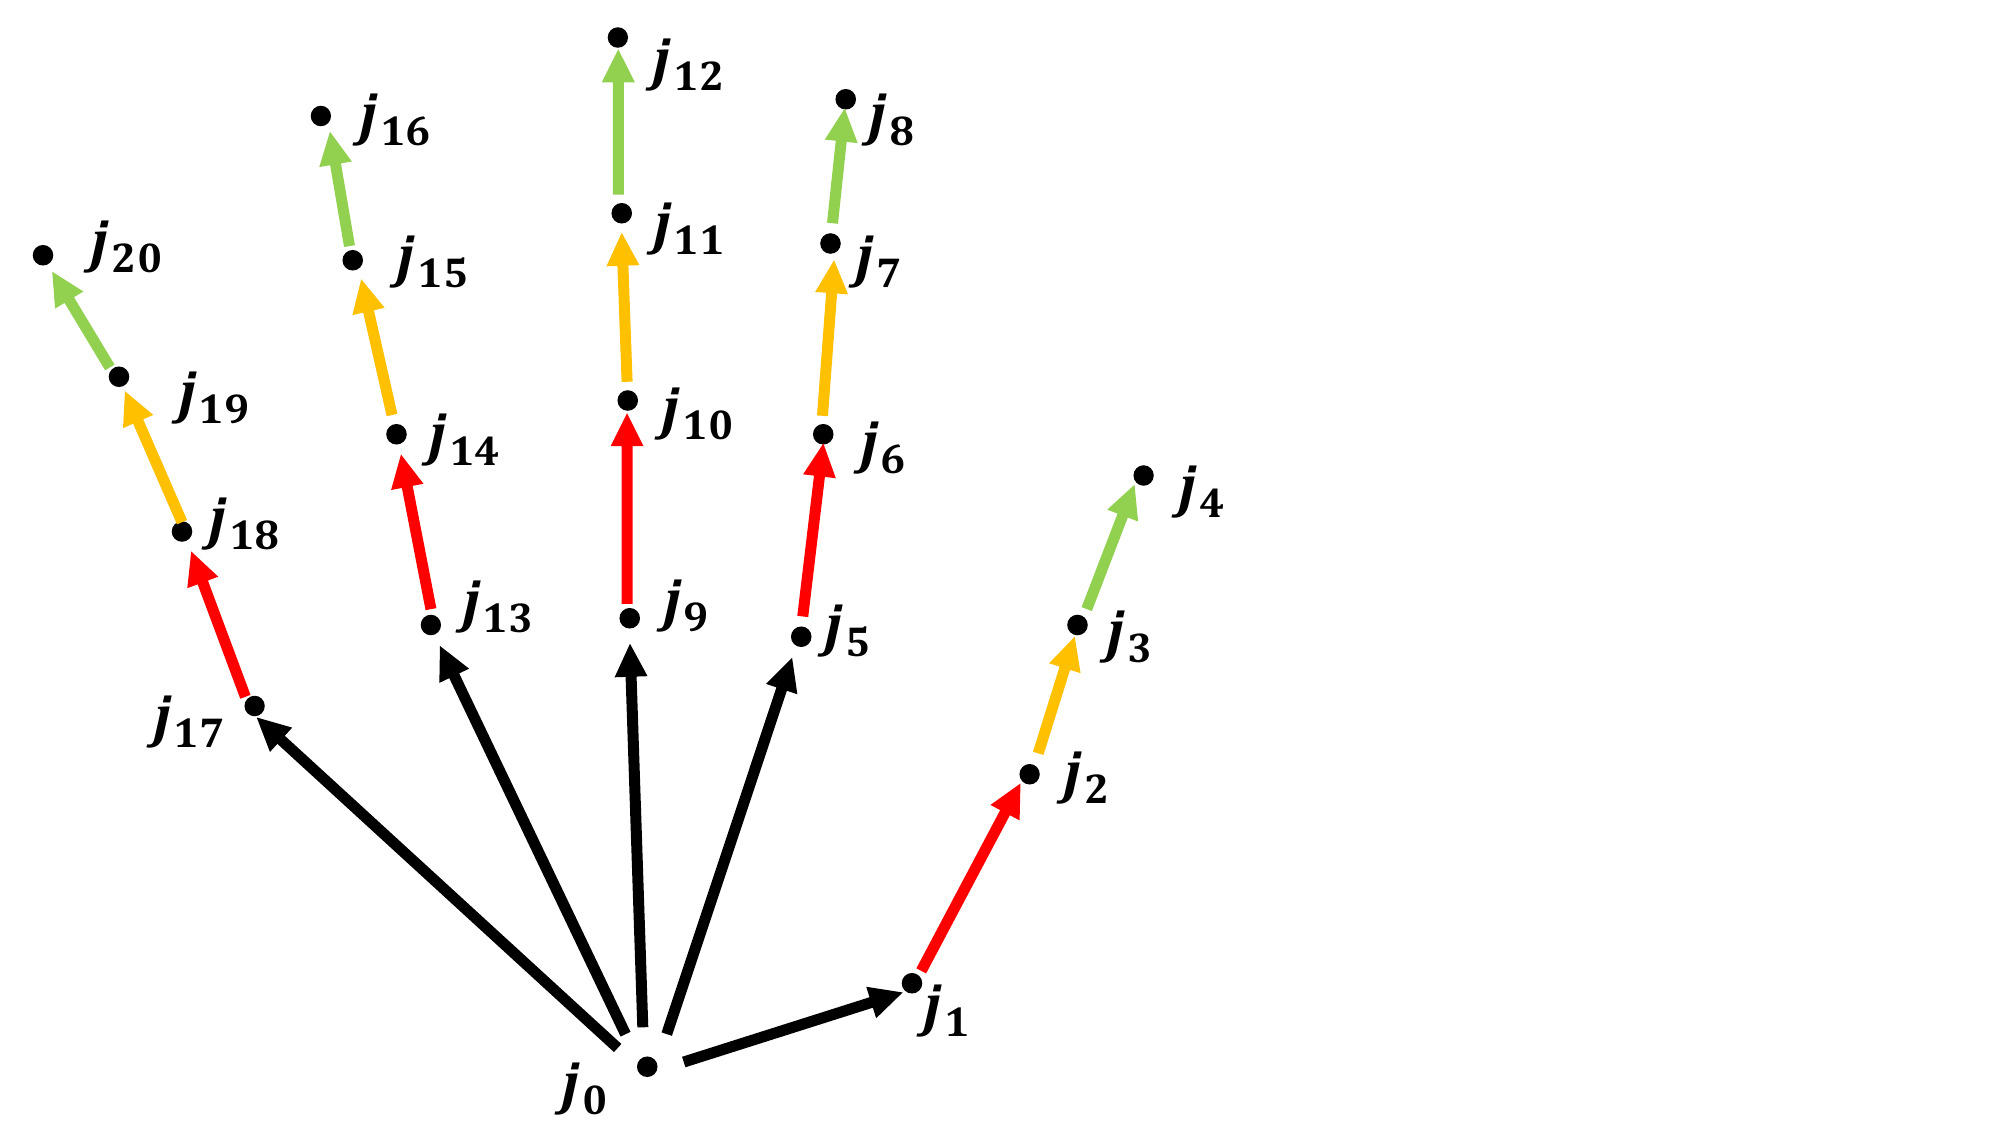}
\caption{The structure of the right hand in our dataset and the input and the output of bone transformation.}
\label{fig:sup_joint}
\end{figure}
